# Supplementary material for: Bounding Transient Moments of Stochastic Chemical Reactions
Source: arXiv:1805.07098 ancillary file (2019-01-06)
Supplement: Supplementary file 1 [file SI.pdf]

# Supporting Information for "Bounding Transient Moments of Stochastic Chemical Reactions"

Yuta Sakurai, Yutaka Hori*

## Implementation details

The implementation of the code was with MATLAB 2016b and SeDuMi 1.32 [1]. Optimization programs were run on HP Z440 workstation with Intel Xeon E5-1650v4 processor (6 cores, 3.60 GHz, 15 MB) and 96 GB of DDR SDRAM (2400 MHz, ECC, Registered).

In the implementation, the variables $\boldsymbol{m}, \boldsymbol{u}, \hat{\boldsymbol{m}}_s$ and $\hat{\boldsymbol{u}}_s$ were normalized by constants to avoid numerical instability. In other words, coefficients in the constraints were multiplied by normalization constants. For the dimerization process, the value of the mean $m_1(t)$ was normalized by 20, and the other moments in $\boldsymbol{m}$ and $\boldsymbol{u}$ were normalized as appropriate ($m_i(t)/20^i$ for the $i$-th moment). This normalization was applied to both YS-SDP (proposed) and GRD-SDP [2]. The temporal moments $\hat{m}_{\boldsymbol{\alpha},s}$ were further normalized by $T$, that is, $\hat{m}_{i,s}(t)/(20^i \times T^s)$. For the dynamic equilibrium reactions, $\boldsymbol{m}$ and $\boldsymbol{u}$ were not normalized. $\hat{\boldsymbol{m}}$ and $\hat{\boldsymbol{u}}$ were normalized by $T$.

*Department of Applied Physics and Physico-Informatics, Keio University, 223-8522 Kanagawa, Japan. Correspondence should be addressed to Yutaka Hori at yhori@appi.keio.ac.jp

# CPU time to solve a single optimization problem

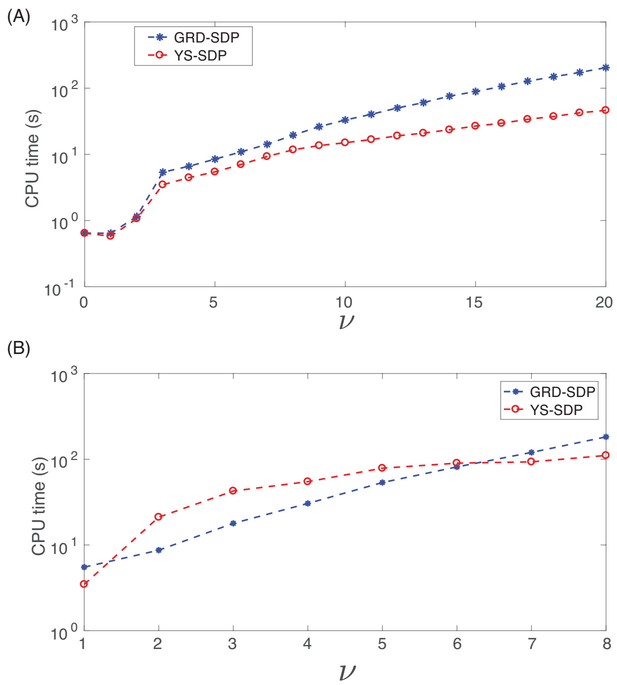


Figure S1: Average CPU time for solving a single optimization problem for a given $T$. (A) Dimerization reaction in Table I. $\mu = 7$ and $n = 1$. (B) Dynamic equilibrium reaction $A + B \xrightarrow{c_1} C \underset{c_3}{\overset{c_2}{\rightleftharpoons}} D$ with the set of parameters and initial conditions used in Fig. 3. $\mu = 3$ and $n = 2$.

# Supplementary numerical examples for Fig. 2(A) and (B)

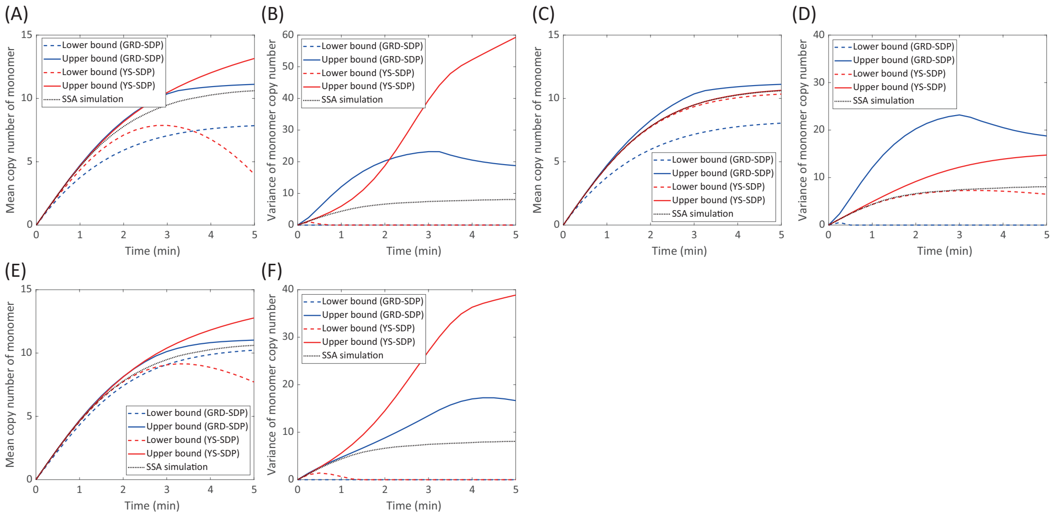


Figure S2: Bounds of the statistics of monomer protein P for different choices of $\mu$ and $\nu$. The model of the reaction is based on Table I. (A), (B): $\mu = 3, \nu = 1$ and $\rho = \{0, -0.8844\}$. (C), (D): $\mu = 3, \nu = 7$ and $\rho = \{0, -0.8844, -1.7481, -2.5902, -3.4099, -4.2062, -4.9778, -5.7231\}$. (E), (F): $\mu = 7, \nu = 1$ and $\rho = \{0, -0.8844\}$. The bounds are computed for $t = 0.25, 0.5, \cdots, 5$.

## A simple irreversible reaction $A + B \to C$

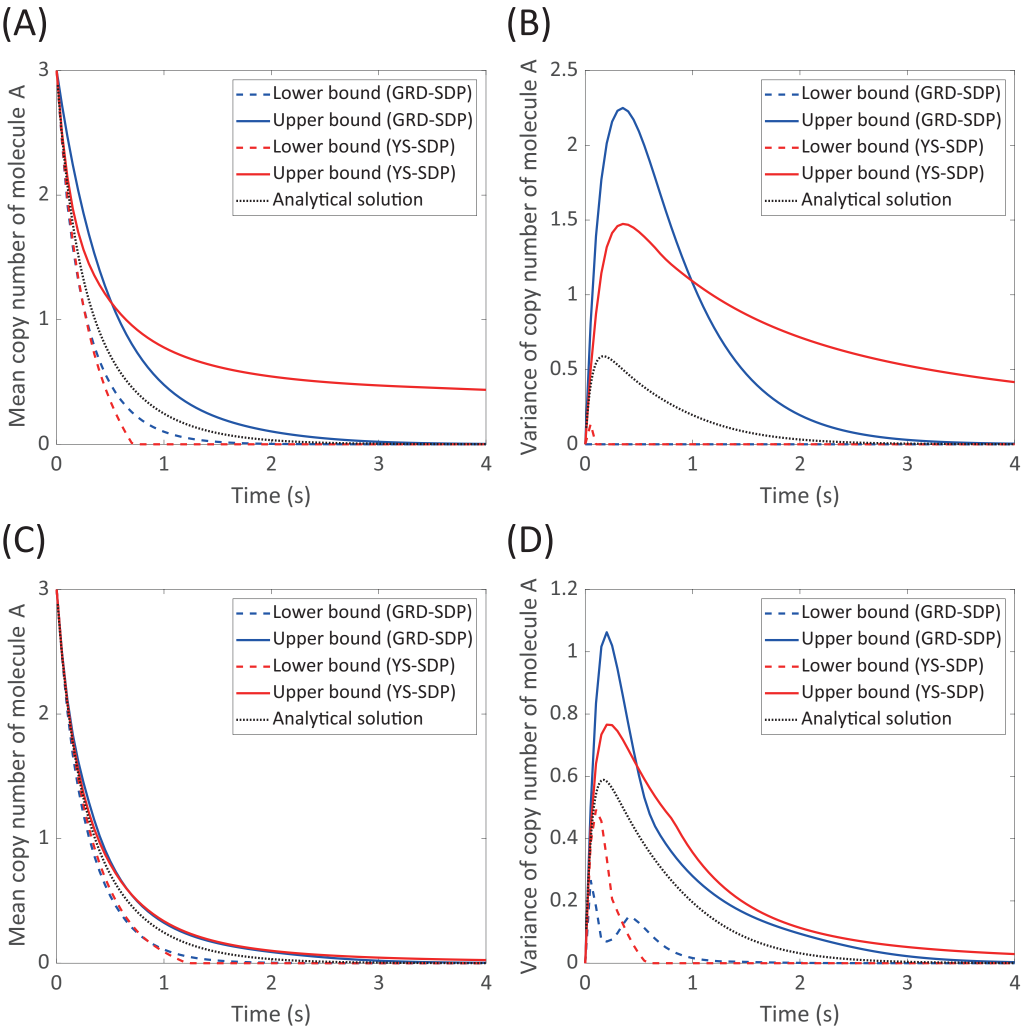


Figure S3: Bounds of the statistics of molecule $A$ for different choices of $\mu$ and $\nu$. The reaction model is $A+B \xrightarrow{c_1} C$, and the parameters and the initial values are set as specified in Fig. 1 and 2 of [2]. (A), (B): $\mu = 3, \nu = 1$ and $\rho = \{0, -2\}$. (C), (D): $\mu = 3, \nu = 2$ and $\rho = \{0, -2, -6\}$. The bounds are computed for $t = 0.05, 0.10, \cdots, 4$.

## A cyclic reaction system $A + B \to C,\ C \to D$ and $D \to A + B$

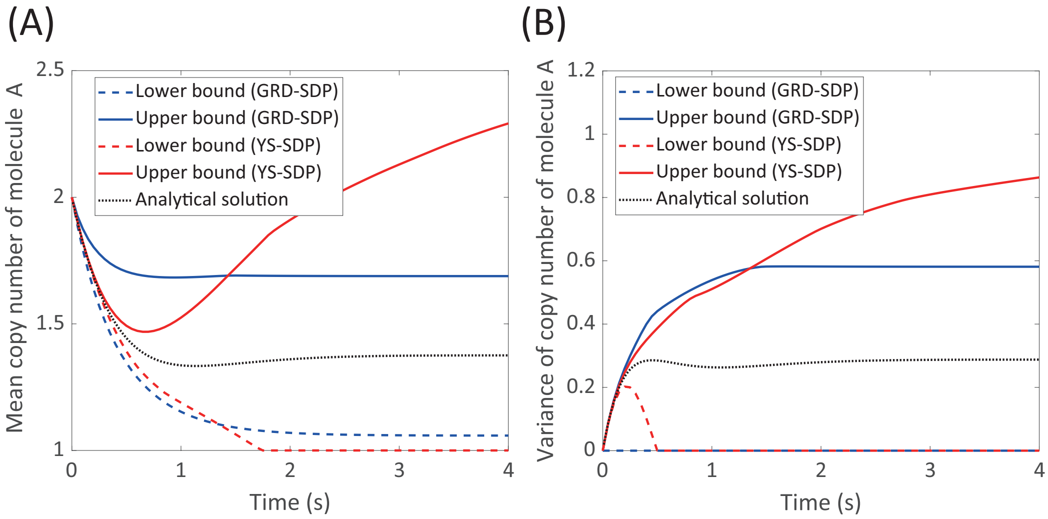


Figure S4: Bounds of the statistics of molecule $A$. The reaction model is $A+B \xrightarrow{c_1} C, C \xrightarrow{c_2} D$ and $D \xrightarrow{c_3} A+B$. The parameters and the initial values are set as specified in Fig. 7 of [2]. (A), (B): $\mu = 3, \nu = 2$ and $\rho = \{0, -2.1322, -4.1637\}$. The bounds are computed for $t = 0.05, 0.10, \cdots, 4$.

## Unimolecular reactions $A \to B \to C$

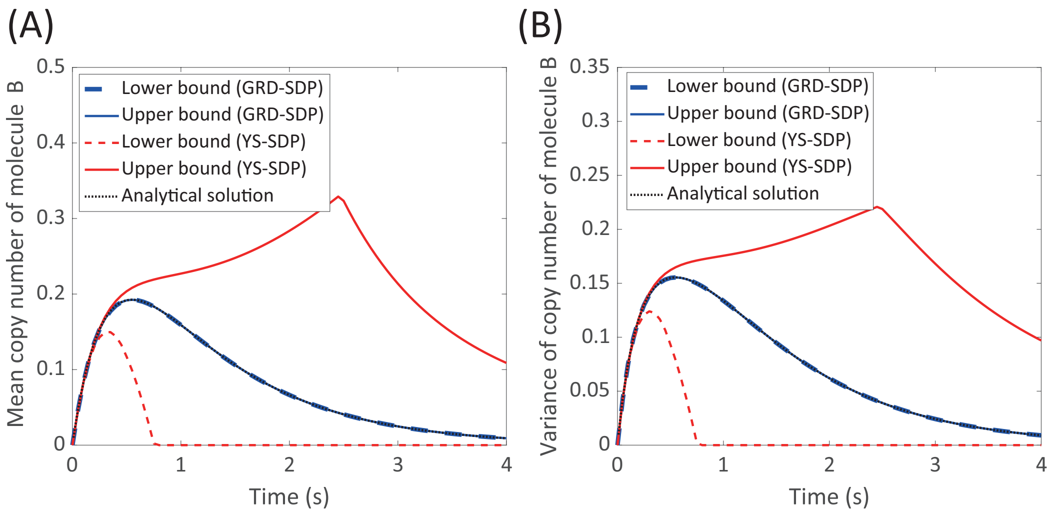


Figure S5: Bounds of the statistics of molecule $B$. The reaction model is $A \xrightarrow{c_1} B$ and $B \xrightarrow{c_2} C$. The parameters are set as specified in Fig. 8 of [2]. The initial values are set $[A, B, C] = [1, 0, 0]$. (A), (B): $\mu = 3, \nu = 2$ and $\rho = \{0, -1, -3\}$. The bounds are computed for $t = 0.05, 0.10, \cdots, 4$

## Supplementary numerical examples for Fig. 3(A), (B)

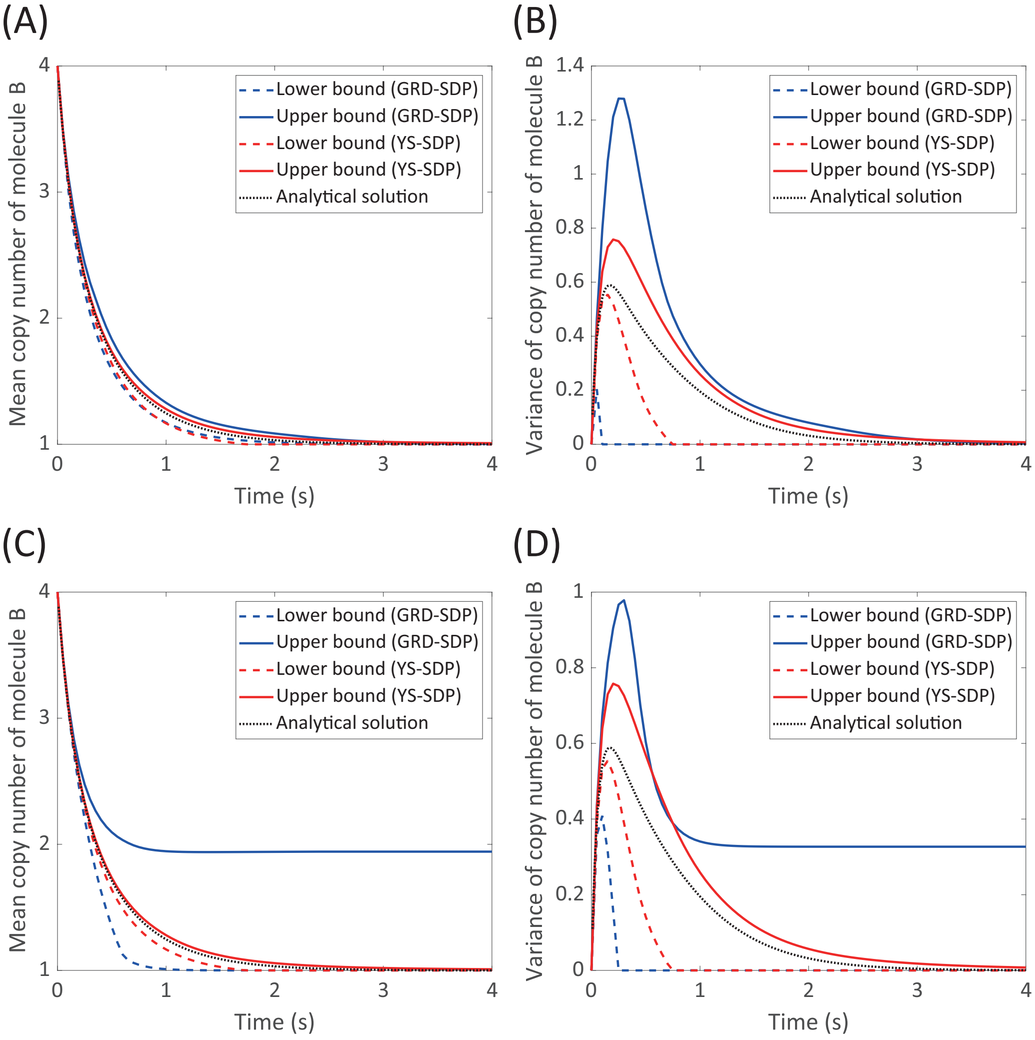


Figure S6: Bounds of the statistics of molecule $B$. The reaction model is $A + B \xrightarrow{c_1} C \underset{c_3}{\overset{c_2}{\rightleftharpoons}} D$. The parameter values and initial conditions are set as specified in Fig. 4 and 6 of [2]. $(A), (B) : \mu = 3, \nu = 3$ and $\rho = \{0, -2, -2.4, -4.4\}$ (see Fig. 4 of [2]). $(C), (D) : \mu = 3, \nu = 3$ and $\rho = \{0, -6, -12, -18\}$ (see Fig. 6 of [2]). The bounds are computed for $t = 0.05, 0.10, \cdots, 4$. Note that the upper bounds of the variance with GRD-SDP is slightly different from those shown in [2] despite our best efforts.

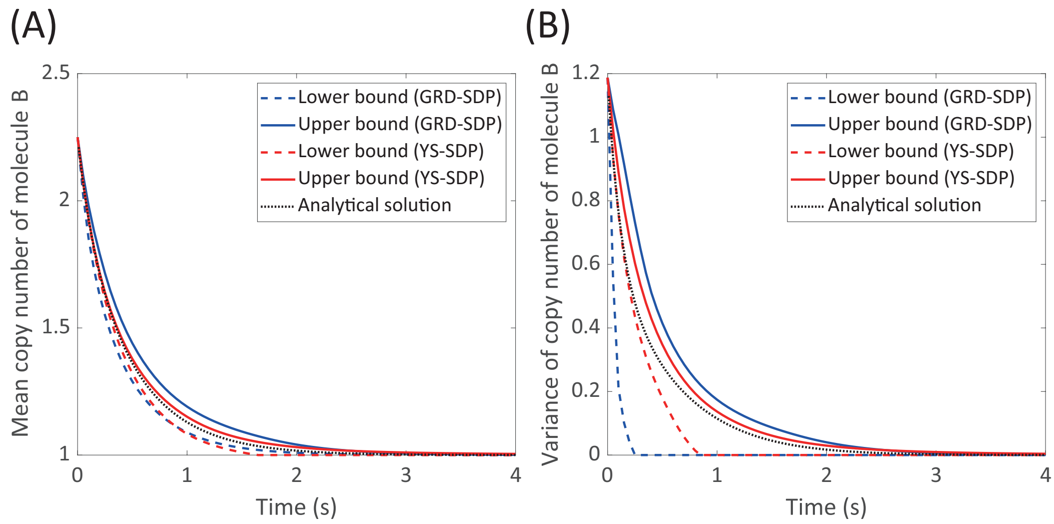


Figure S7: Bounds of the statistics of molecule $B$. The reaction model is $A + B \xrightarrow{c_1} C \underset{c_3}{\overset{c_2}{\rightleftharpoons}} D$. The parameter values and initial conditions are set as specified in Fig. 9 of [2]. $(A),(B) : \mu = 3, \nu = 3$ and $\rho = \{0, -2, -2.4, -4.4\}$. The initial values are set $P_{[3,4,0,0]} = 1/4, P_{[1,2,2,0]} = 1/2, P_{[0,1,0,3]} = 1/4$ and $P_{\boldsymbol{x}}(0) = 0$ for all the other possible states. The bounds are computed for $t = 0.05, 0.10, \cdots, 4$.

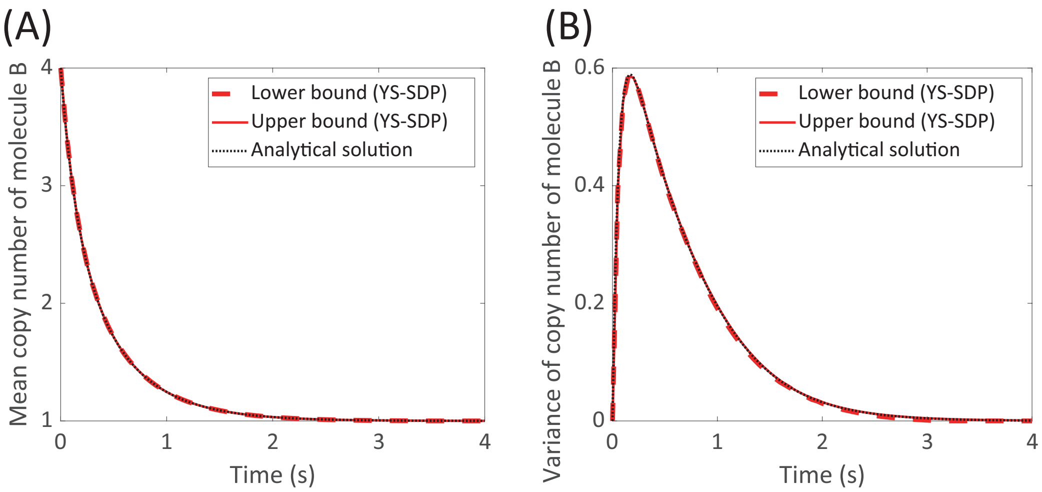


Figure S8: Tight bounds are obtained for the example shown in Fig. 3 by using larger values of $\mu$ and $\nu$ ($\mu = 7$ and $\nu = 6$). The reaction model is $A + B \xrightarrow{c_1} C \underset{c_3}{\overset{c_2}{\rightleftharpoons}} D$. The parameter values and initial conditions are set equal to those in Fig. 3. The bounds are computed for $t = 0.05, 0.10, \cdots, 4$. For all $t \in [0, 4]$, the gap between the upper/lower bounds and the analytic solution is within $\pm 0.0015$ for the mean and $\pm 0.0045$ for the variance, implying that the bounds become sufficiently tight for practical use by increasing $\mu$ and $\nu$.

# References

[1] J. F. Sturm, "Using SeDuMi 1.02, a MATLAB toolbox for optimization over symmetric cones," *Optimization Methods and Software*, vol. 11–12, pp. 625–653, 1999.

[2] G. R. Dowdy and P. I. Barton, "Dynamic bounds on stochastic chemical kinetic systems using semidefinite programming," 2018, arXiv:1802.04409v2 (available at http://arxiv.org/abs/1802.04409v2).
